# Supplementary material for: Defending against Reconstruction Attack in Vertical Federated Learning
Source: arXiv:2107.09898 source file (2021-07-21)
Supplement: Supplementary file 1 [file appendix.tex]

\section{Distance Correlation Related}
dCor is sensitive to the batch sizes. To demonstrate this observation, we compute the dCor between $X$\footnote{$X$ is a $n$ by $384$ matrix from a real CVR dataset. More details of the corresponding dataset can be seen at the Experimental section.} and random Gaussian noise with different batch sizes. As shown in Figure ~\ref{fig:dcor_X_random_noise_batch_sizes}, a larger batch size can give a more accurate estimation of the distance correlation, since $\mathcal{X}$ contains meaningful information and should have small distance correlation with random noise.

\begin{figure}[h!]
    \centering
    \includegraphics[width=0.5\textwidth]{figures/distance_correlation/dcor_X_random_noise_batch_sizes.pdf}
    \caption{Distance correlation (dCor) between $\mathcal{X}$ and random Gaussian noise with different batch sizes. dCor is sensitive to batch sizes. A larger batch size can give a more accurate estimation of dCor.}
    \label{fig:dcor_X_random_noise_batch_sizes}
\end{figure}

\begin{figure*}[ht!]
  \begin{minipage}[b]{0.33\linewidth}
  \centering
    \includegraphics[width=\linewidth]{figures/distance_correlation/minizing_dcor_only_dcor_activation.pdf}
    \caption*{(a)}
  \end{minipage}
  \begin{minipage}[b]{0.33\linewidth}
  \centering
    \includegraphics[width=\linewidth]{figures/distance_correlation/minizing_dcor_only_roc_auc.pdf}
    \caption*{(b)}
  \end{minipage}
  \begin{minipage}[b]{0.33\linewidth}
  \centering
    \includegraphics[width=\linewidth]{figures/distance_correlation/logdcor_batch_sizes.pdf}
    \caption*{(c)}
  \end{minipage}
 \caption{Figure (a) shows the distance correlation between $\mathcal{X}$ and the cut layer embedding $\mathcal{F(X)}$ with different values of distance correlation weights ($\alpha_d = [0, 0.01, 0.1, 0.15]$). Figure (b) shows the corresponding model performance. $logdcor$ represents that we use $log(dCor(\mathcal{X}, \mathcal{F(X)}))$ in the loss function. Figure (c) shows the distance correlation between $\mathcal{X}$ and the cut layer embedding $\mathcal{F(X)}$ with different batch sizes. logdcor\_$\alpha_d$\_bs\_$n$ represents that we use $log(dCor(\mathcal{X}, \mathcal{F(X)}))$ in the loss function with corresponding weight $\alpha_d$ and the batch size is $n$.}
 \label{fig:minimizing_dcor_only} 
\end{figure*}
